# Supplementary material for: First Measurement of Differential Cross Sections for Muon Neutrino Charged Current Interactions on Argon with a Two-proton Final State in the MicroBooNE Detector
Source: arXiv:2211.03734 ancillary file (2025-02-25)
Supplement: Supplementary file 1 [file CC2p_PRL__Supplemental_Materials.pdf]

# Supplemental Materials: First Measurement of Differential Cross Sections for Muon Neutrino Charged Current Interactions on Argon with a Two Proton Final State in the MicroBooNE Detector

August 3, 2023

## CROSS SECTION VALUES

Tables 1, 2, and 3 include the single differential cross sections as a function of the cosine of the opening angle between the protons,  $\cos(\gamma_{\vec{p}_L, \vec{p}_R})$ , the cosine of the opening angle between the muon momentum vector and the total proton momentum vector,  $\cos(\gamma_{\vec{p}_\mu, \vec{p}_{\text{sum}}})$ , and the magnitude of the transverse momentum of the muon and two proton system ( $\delta P_T$ ), respectively. Tables 4, 6, and 8 include the single differential cross sections as a function of the momentum of the muon,  $P_\mu$ , leading proton,  $P_L$ , and recoil proton,  $P_R$ , respectively. Tables 5, 7, and 9 include the single differential cross-sections as a function of the cosine of the opening angle with respect to the beam of the muon, leading proton, and recoil proton, respectively.

| Bin Number | $\cos(\gamma_{\vec{p}_L, \vec{p}_R})$<br>Range | $d\sigma/d\cos(\gamma_{\vec{p}_L, \vec{p}_R})$<br>[ $10^{-38}\text{cm}^2$ ] | Statistical<br>Uncertainty<br>[ $10^{-38}\text{cm}^2$ ] | Systematic<br>Uncertainty<br>[ $10^{-38}\text{cm}^2$ ] | Total<br>Uncertainty<br>[ $10^{-38}\text{cm}^2$ ] |
|------------|------------------------------------------------|-----------------------------------------------------------------------------|---------------------------------------------------------|--------------------------------------------------------|---------------------------------------------------|
| 1          | [ -1.00 , -0.75 )                              | 1.43                                                                        | 0.19                                                    | 0.44                                                   | 0.47                                              |
| 2          | [ -0.75 , -0.50 )                              | 1.32                                                                        | 0.18                                                    | 0.52                                                   | 0.55                                              |
| 3          | [ -0.50 , -0.25 )                              | 1.73                                                                        | 0.19                                                    | 0.49                                                   | 0.52                                              |
| 4          | [ -0.25 , 0.00 )                               | 1.68                                                                        | 0.18                                                    | 0.71                                                   | 0.73                                              |
| 5          | [ 0.00 , 0.25 )                                | 1.54                                                                        | 0.17                                                    | 0.78                                                   | 0.79                                              |
| 6          | [ 0.25 , 0.50 )                                | 1.33                                                                        | 0.16                                                    | 0.62                                                   | 0.64                                              |
| 7          | [ 0.50 , 0.75 )                                | 0.99                                                                        | 0.14                                                    | 0.23                                                   | 0.27                                              |
| 8          | [ 0.75 , 1.00 )                                | 0.67                                                                        | 0.16                                                    | 0.49                                                   | 0.51                                              |

Table 1: Differential charged current two proton differential cross-sections per argon nucleus as a function of the cosine of the opening angle between the two protons,  $\cos(\gamma_{\vec{p}_L, \vec{p}_R})$ .

| Bin<br>Number | $\cos(\gamma_{\vec{P}_\mu, \vec{P}_{\text{sum}}})$<br>Range | $d\sigma/d\cos(\gamma_{\vec{P}_\mu, \vec{P}_{\text{sum}}})$<br>[ $10^{-38}\text{cm}^2$ ] | Statistical<br>Uncertainty<br>[ $10^{-38}\text{cm}^2$ ] | Systematic<br>Uncertainty<br>[ $10^{-38}\text{cm}^2$ ] | Total<br>Uncertainty<br>[ $10^{-38}\text{cm}^2$ ] |
|---------------|-------------------------------------------------------------|------------------------------------------------------------------------------------------|---------------------------------------------------------|--------------------------------------------------------|---------------------------------------------------|
| 1             | [ -1.00 , -0.75 )                                           | 1.14                                                                                     | 0.20                                                    | 0.39                                                   | 0.44                                              |
| 2             | [ -0.75 , -0.50 )                                           | 1.30                                                                                     | 0.19                                                    | 0.42                                                   | 0.46                                              |
| 3             | [ -0.50 , -0.25 )                                           | 1.69                                                                                     | 0.21                                                    | 0.67                                                   | 0.70                                              |
| 4             | [ -0.25 , 0.00 )                                            | 1.72                                                                                     | 0.21                                                    | 0.41                                                   | 0.46                                              |
| 5             | [ 0.00 , 0.25 )                                             | 1.94                                                                                     | 0.24                                                    | 0.96                                                   | 0.99                                              |
| 6             | [ 0.25 , 0.50 )                                             | 1.27                                                                                     | 0.23                                                    | 0.69                                                   | 0.73                                              |
| 7             | [ 0.50 , 0.75 )                                             | 1.057                                                                                    | 0.21                                                    | 0.36                                                   | 0.42                                              |
| 8             | [ 0.75 , 1.00 )                                             | 0.66                                                                                     | 0.17                                                    | 0.38                                                   | 0.41                                              |

Table 2: Differential charged current two proton differential cross-sections per argon nucleus as a function of the cosine of the angle between the muon momentum vector and the total proton momentum vector,  $\cos(\gamma_{\vec{P}_\mu, \vec{P}_{\text{sum}}})$ .

| Bin<br>Number | $\delta P_T$ Range<br>[GeV/c] | $d\sigma/d\delta P_T$<br>[ $10^{-38}\text{cm}^2/(\text{GeV}/c)$ ] | Statistical<br>Uncertainty<br>[ $10^{-38}\text{cm}^2/(\text{GeV}/c)$ ] | Systematic<br>Uncertainty<br>[ $10^{-38}\text{cm}^2/(\text{GeV}/c)$ ] | Total<br>Uncertainty<br>[ $10^{-38}\text{cm}^2/(\text{GeV}/c)$ ] |
|---------------|-------------------------------|-------------------------------------------------------------------|------------------------------------------------------------------------|-----------------------------------------------------------------------|------------------------------------------------------------------|
| 1             | [ 0.00 , 0.10 )               | 2.15                                                              | 0.24                                                                   | 0.52                                                                  | 0.57                                                             |
| 2             | [ 0.10 , 0.20 )               | 5.00                                                              | 0.41                                                                   | 1.28                                                                  | 1.35                                                             |
| 3             | [ 0.20 , 0.30 )               | 6.06                                                              | 0.42                                                                   | 1.53                                                                  | 1.59                                                             |
| 4             | [ 0.30 , 0.40 )               | 4.63                                                              | 0.38                                                                   | 1.15                                                                  | 1.21                                                             |
| 5             | [ 0.40 , 0.50 )               | 3.11                                                              | 0.30                                                                   | 1.00                                                                  | 1.04                                                             |
| 6             | [ 0.50 , 0.60 )               | 2.45                                                              | 0.31                                                                   | 0.85                                                                  | 0.90                                                             |
| 7             | [ 0.60 , 1.00 )               | 0.87                                                              | 0.12                                                                   | 0.31                                                                  | 0.33                                                             |

Table 3: Differential charged current two proton differential cross-sections per argon nucleus as a function of the magnitude of the transverse momentum of the muon and two proton system,  $\delta P_T$ .

| Bin<br>Number | $P_\mu$ Range<br>[Gev/c] | $d\sigma/dP_\mu$<br>[ $10^{-38}\text{cm}^2/(\text{GeV}/c)$ ] | Statistical<br>Uncertainty<br>[ $10^{-38}\text{cm}^2/(\text{GeV}/c)$ ] | Systematic<br>Uncertainty<br>[ $10^{-38}\text{cm}^2/(\text{GeV}/c)$ ] | Total<br>Uncertainty<br>[ $10^{-38}\text{cm}^2/(\text{GeV}/c)$ ] |
|---------------|--------------------------|--------------------------------------------------------------|------------------------------------------------------------------------|-----------------------------------------------------------------------|------------------------------------------------------------------|
| 1             | [ 0.10 , 0.30 )          | 2.88                                                         | 0.27                                                                   | 1.18                                                                  | 1.21                                                             |
| 2             | [ 0.30 , 0.50 )          | 4.0                                                          | 0.29                                                                   | 1.11                                                                  | 1.14                                                             |
| 3             | [ 0.50 , 0.70 )          | 2.95                                                         | 0.24                                                                   | 0.77                                                                  | 0.81                                                             |
| 4             | [ 0.70 , 0.90 )          | 2.10                                                         | 0.21                                                                   | 0.67                                                                  | 0.69                                                             |
| 5             | [ 0.90 , 1.20 )          | 0.83                                                         | 0.15                                                                   | 0.42                                                                  | 0.45                                                             |

Table 4: Differential charged current two proton differential cross-sections per argon nucleus as a function of the muon momentum,  $P_\mu$ .

| Bin<br>Number | $\cos(\theta_\mu)$<br>Range | $d\sigma/d\cos(\theta_\mu)$<br>[ $10^{-38}\text{cm}^2$ ] | Statistical<br>Uncertainty<br>[ $10^{-38}\text{cm}^2$ ] | Systematic<br>Uncertainty<br>[ $10^{-38}\text{cm}^2$ ] | Total<br>Uncertainty<br>[ $10^{-38}\text{cm}^2$ ] |
|---------------|-----------------------------|----------------------------------------------------------|---------------------------------------------------------|--------------------------------------------------------|---------------------------------------------------|
| 1             | [ -1.00 , -0.75 )           | 0.33                                                     | 0.12                                                    | 0.27                                                   | 0.30                                              |
| 2             | [ -0.75 , -0.50 )           | 0.36                                                     | 0.09                                                    | 0.11                                                   | 0.15                                              |
| 3             | [ -0.50 , -0.25 )           | 0.51                                                     | 0.09                                                    | 0.41                                                   | 0.42                                              |
| 4             | [ -0.25 , 0.00 )            | 0.89                                                     | 0.13                                                    | 0.18                                                   | 0.22                                              |
| 5             | [ 0.00 , 0.25 )             | 1.05                                                     | 0.14                                                    | 0.43                                                   | 0.45                                              |
| 6             | [ 0.25 , 0.50 )             | 1.70                                                     | 0.17                                                    | 0.69                                                   | 0.72                                              |
| 7             | [ 0.50 , 0.75 )             | 2.62                                                     | 0.22                                                    | 0.61                                                   | 0.65                                              |
| 8             | [ 0.75 , 1.00 )             | 3.46                                                     | 0.33                                                    | 1.41                                                   | 1.45                                              |

Table 5: Differential charged current two proton differential cross-sections per argon nucleus as a function of the cosine of the angle relative to the beam direction of the muon,  $\cos(\theta_\mu)$ .

| Bin<br>Number | $P_L$ Range<br>[GeV/c] | $d\sigma/dP_L$<br>[ $10^{-38}\text{cm}^2/(\text{GeV}/c)$ ] | Statistical<br>Uncertainty<br>[ $10^{-38}\text{cm}^2/(\text{GeV}/c)$ ] | Systematic<br>Uncertainty<br>[ $10^{-38}\text{cm}^2/(\text{GeV}/c)$ ] | Total<br>Uncertainty<br>[ $10^{-38}\text{cm}^2/(\text{GeV}/c)$ ] |
|---------------|------------------------|------------------------------------------------------------|------------------------------------------------------------------------|-----------------------------------------------------------------------|------------------------------------------------------------------|
| 1             | [ 0.30 , 0.40 )        | 5.67                                                       | 1.18                                                                   | 3.61                                                                  | 3.79                                                             |
| 2             | [ 0.40 , 0.50 )        | 5.59                                                       | 0.65                                                                   | 1.78                                                                  | 1.90                                                             |
| 3             | [ 0.50 , 0.60 )        | 5.52                                                       | 0.56                                                                   | 2.72                                                                  | 2.77                                                             |
| 4             | [ 0.60 , 0.70 )        | 4.87                                                       | 0.50                                                                   | 1.26                                                                  | 1.36                                                             |
| 5             | [ 0.70 , 0.80 )        | 3.72                                                       | 0.40                                                                   | 0.76                                                                  | 0.86                                                             |
| 6             | [ 0.80 , 1.00 )        | 2.01                                                       | 0.21                                                                   | 0.53                                                                  | 0.57                                                             |

Table 6: Differential charged current two proton differential cross-sections per argon nucleus as a function of the leading proton momentum,  $P_L$ .

| Bin<br>Number | $\cos(\theta_L)$<br>Range | $d\sigma/d\cos(\theta_L)$<br>[ $10^{-38}\text{cm}^2$ ] | Statistical<br>Uncertainty<br>[ $10^{-38}\text{cm}^2$ ] | Systematic<br>Uncertainty<br>[ $10^{-38}\text{cm}^2$ ] | Total<br>Uncertainty<br>[ $10^{-38}\text{cm}^2$ ] |
|---------------|---------------------------|--------------------------------------------------------|---------------------------------------------------------|--------------------------------------------------------|---------------------------------------------------|
| 1             | [ -1.00 , -0.75 )         | 0.25                                                   | 0.10                                                    | 0.23                                                   | 0.25                                              |
| 2             | [ -0.75 , -0.50 )         | 0.26                                                   | 0.09                                                    | 0.24                                                   | 0.26                                              |
| 3             | [ -0.50 , -0.25 )         | 0.40                                                   | 0.11                                                    | 0.19                                                   | 0.22                                              |
| 4             | [ -0.25 , 0.00 )          | 0.54                                                   | 0.14                                                    | 0.26                                                   | 0.29                                              |
| 5             | [ 0.00 , 0.25 )           | 1.20                                                   | 0.19                                                    | 0.58                                                   | 0.61                                              |
| 6             | [ 0.25 , 0.50 )           | 1.74                                                   | 0.20                                                    | 0.86                                                   | 0.88                                              |
| 7             | [ 0.50 , 0.75 )           | 2.49                                                   | 0.23                                                    | 0.77                                                   | 0.80                                              |
| 8             | [ 0.75 , 1.00 )           | 3.79                                                   | 0.29                                                    | 1.17                                                   | 1.20                                              |

Table 7: Differential charged current two proton differential cross-sections per argon nucleus as a function of the cosine of the angle relative to the beam direction of the leading proton,  $\cos(\theta_L)$ .

| Bin<br>Number | $P_R$ Range<br>[GeV/c] | $d\sigma/dP_R$<br>[ $10^{-38}\text{cm}^2/(\text{GeV}/c)$ ] | Statistical<br>Uncertainty<br>[ $10^{-38}\text{cm}^2/(\text{GeV}/c)$ ] | Systematic<br>Uncertainty<br>[ $10^{-38}\text{cm}^2/(\text{GeV}/c)$ ] | Total<br>Uncertainty<br>[ $10^{-38}\text{cm}^2/(\text{GeV}/c)$ ] |
|---------------|------------------------|------------------------------------------------------------|------------------------------------------------------------------------|-----------------------------------------------------------------------|------------------------------------------------------------------|
| 1             | [ 0.30 , 0.40 )        | 15.9                                                       | 1.25                                                                   | 5.55                                                                  | 5.69                                                             |
| 2             | [ 0.40 , 0.50 )        | 7.22                                                       | 0.55                                                                   | 2.12                                                                  | 2.19                                                             |
| 3             | [ 0.50 , 0.60 )        | 3.02                                                       | 0.34                                                                   | 0.86                                                                  | 0.93                                                             |
| 4             | [ 0.60 , 0.70 )        | 1.07                                                       | 0.16                                                                   | 0.29                                                                  | 0.33                                                             |
| 5             | [ 0.70 , 0.80 )        | 0.33                                                       | 0.09                                                                   | 0.14                                                                  | 0.17                                                             |
| 6             | [ 0.80 , 1.00 )        | 0.11                                                       | 0.05                                                                   | 0.07                                                                  | 0.09                                                             |

Table 8: Differential charged current two proton differential cross-sections per argon nucleus as a function of the recoil proton momentum,  $P_R$ .

| Bin<br>Number | $\cos(\theta_R)$<br>Range | $d\sigma/d\cos(\theta_R)$<br>[ $10^{-38}\text{cm}^2$ ] | Statistical<br>Uncertainty<br>[ $10^{-38}\text{cm}^2$ ] | Systematic<br>Uncertainty<br>[ $10^{-38}\text{cm}^2$ ] | Total<br>Uncertainty<br>[ $10^{-38}\text{cm}^2$ ] |
|---------------|---------------------------|--------------------------------------------------------|---------------------------------------------------------|--------------------------------------------------------|---------------------------------------------------|
| 1             | [ -1.00 , -0.75 )         | 0.51                                                   | 0.11                                                    | 0.35                                                   | 0.36                                              |
| 2             | [ -0.75 , -0.50 )         | 0.67                                                   | 0.11                                                    | 0.34                                                   | 0.38                                              |
| 3             | [ -0.50 , -0.25 )         | 0.87                                                   | 0.13                                                    | 0.54                                                   | 0.55                                              |
| 4             | [ -0.25 , 0.00 )          | 1.09                                                   | 0.17                                                    | 0.44                                                   | 0.47                                              |
| 5             | [ 0.00 , 0.25 )           | 1.31                                                   | 0.18                                                    | 0.67                                                   | 0.69                                              |
| 6             | [ 0.25 , 0.50 )           | 1.84                                                   | 0.20                                                    | 0.67                                                   | 0.70                                              |
| 7             | [ 0.50 , 0.75 )           | 1.87                                                   | 0.20                                                    | 0.67                                                   | 0.70                                              |
| 8             | [ 0.75 , 1.00 )           | 2.51                                                   | 0.24                                                    | 0.62                                                   | 0.67                                              |

Table 9: Differential charged current two proton differential cross-sections per argon nucleus as a function of the cosine of the angle relative to the beam direction of the recoil proton,  $\cos(\theta_R)$ .

## TOTAL COVARIANCE AND CORRELATION MATRICES

Figures 1, 2, and 3 display the covariance and correlation matrices for the cosine of the opening angle between the protons,  $\cos(\gamma_{\vec{p}_L, \vec{p}_R})$ , the cosine of the opening angle between the muon momentum vector and the total proton momentum vector,  $\cos(\gamma_{\vec{p}_\mu, \vec{p}_{\text{sum}}})$ , and the magnitude of the transverse momentum of the muon and two proton system,  $\delta P_T$ , respectively. Figures 4, 5, and 6 display the total covariance matrices for the (a) momentum and (b) angle with respect to the beam,  $\cos(\theta)$ , of the muon, leading proton, and recoil proton, respectively.

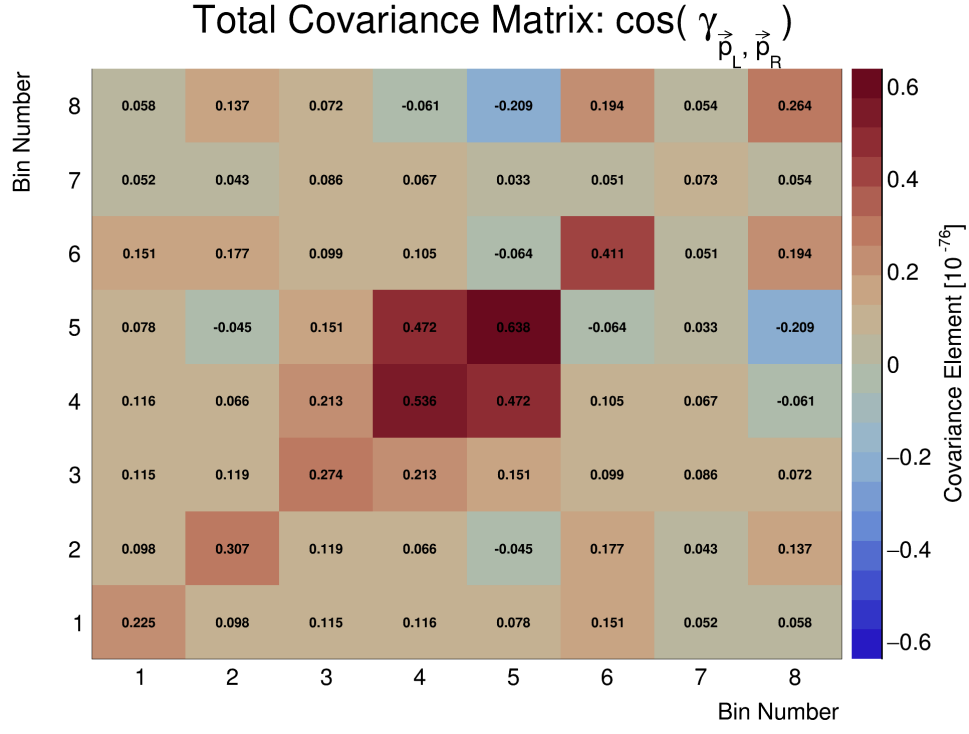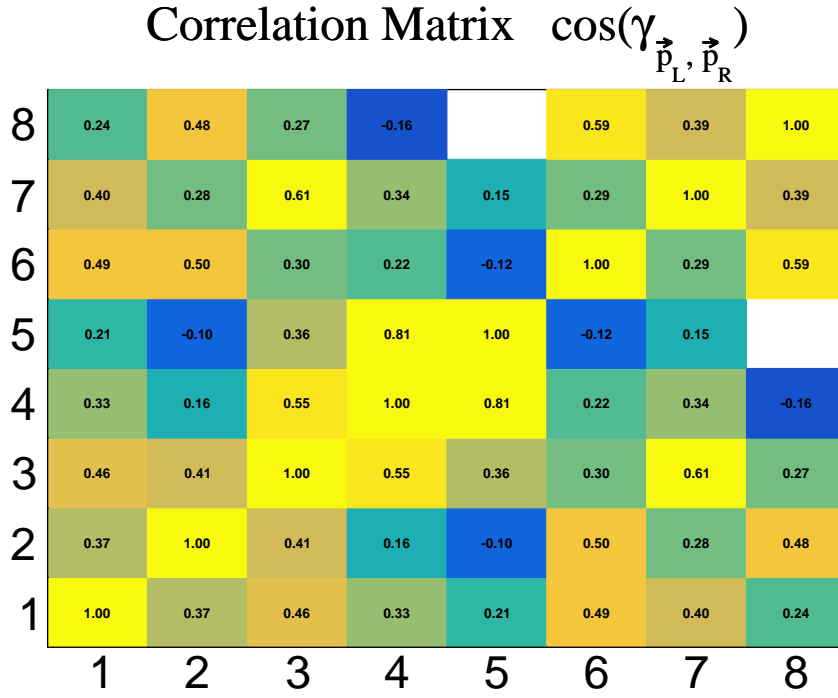

Figure 1: Covariance (top) and correlation (bottom) matrices for the cosine of the opening angle between the protons,  $\cos(\gamma_{\vec{p}_L, \vec{p}_R})$ .

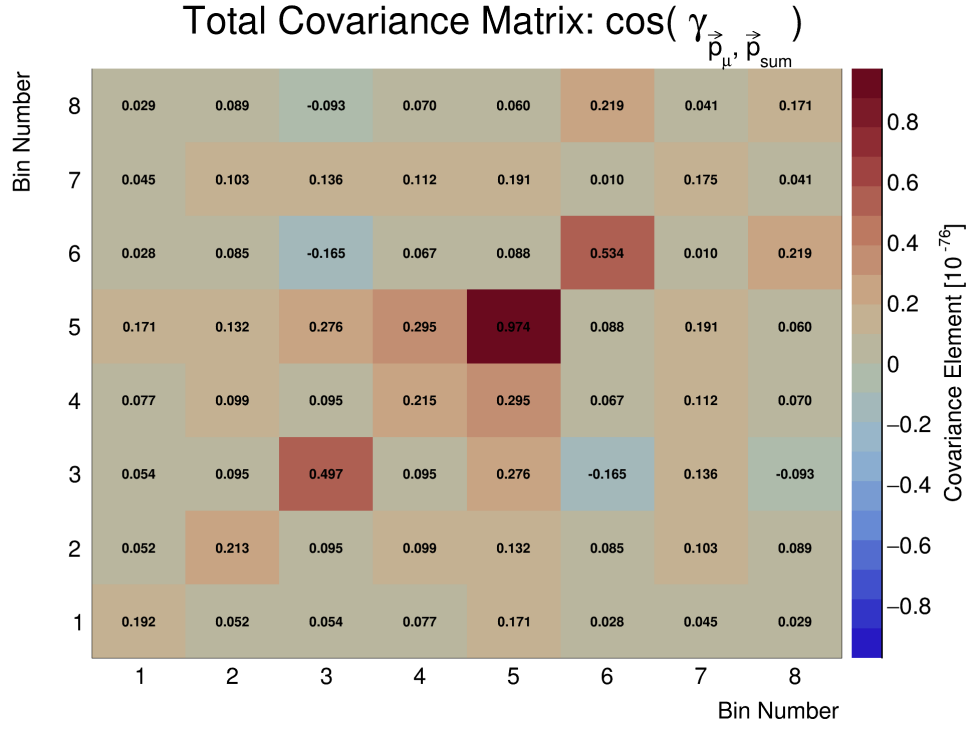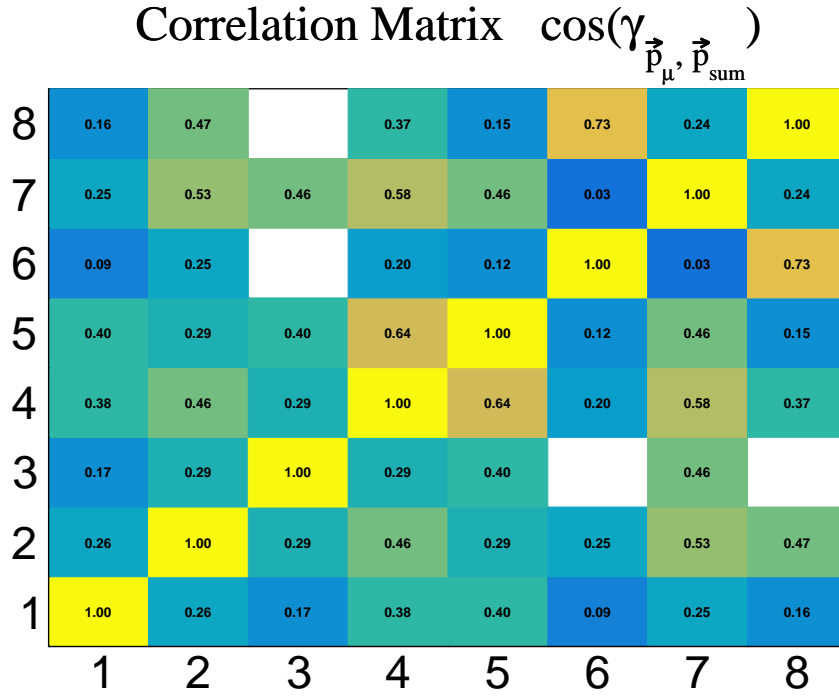

Figure 2: Covariance (top) and correlation (bottom) matrices for the cosine of the opening angle between the muon momentum vector and the total proton momentum vector,  $\cos(\gamma_{\vec{p}_\mu, \vec{p}_{\text{sum}}})$ .

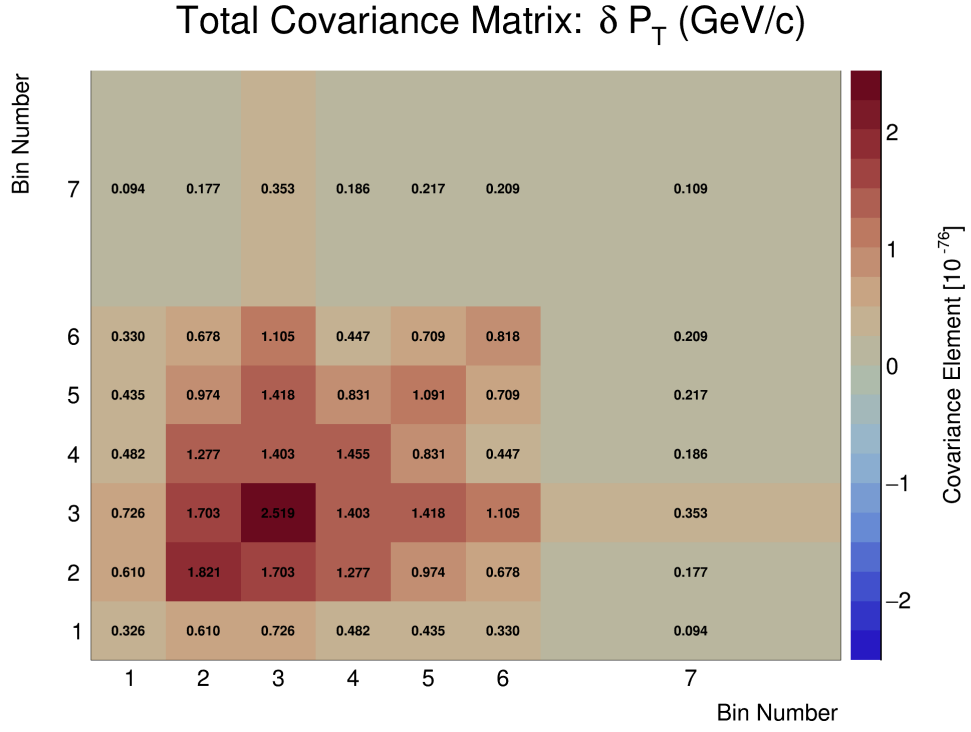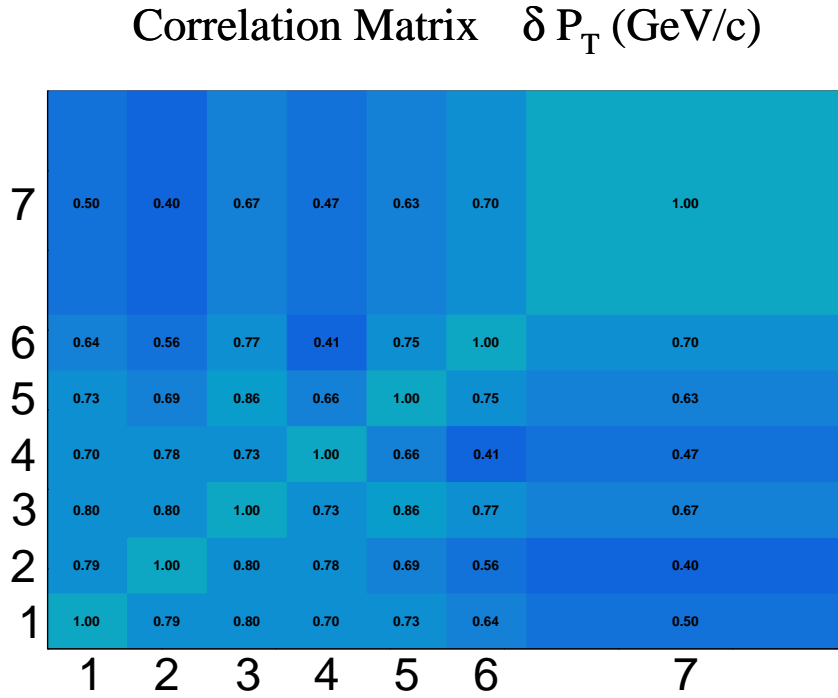

Figure 3: Covariance (top) and correlation (bottom) matrices for the magnitude of the transverse momentum of the muon and two proton system,  $\delta P_T$ .

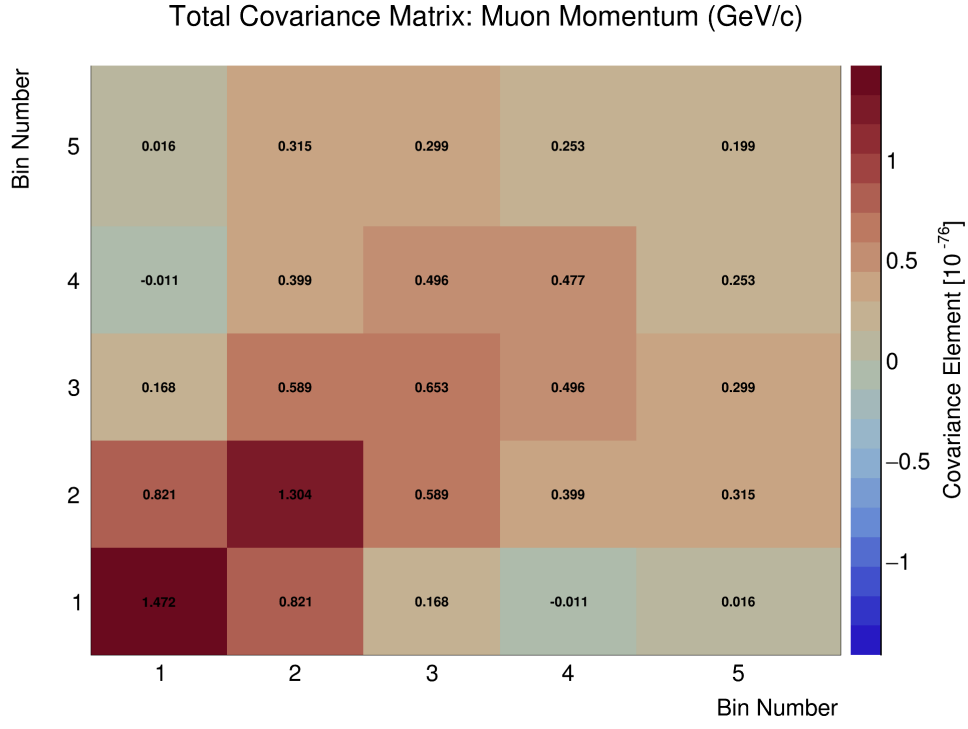

(a) Muon Momentum,  $P_\mu$

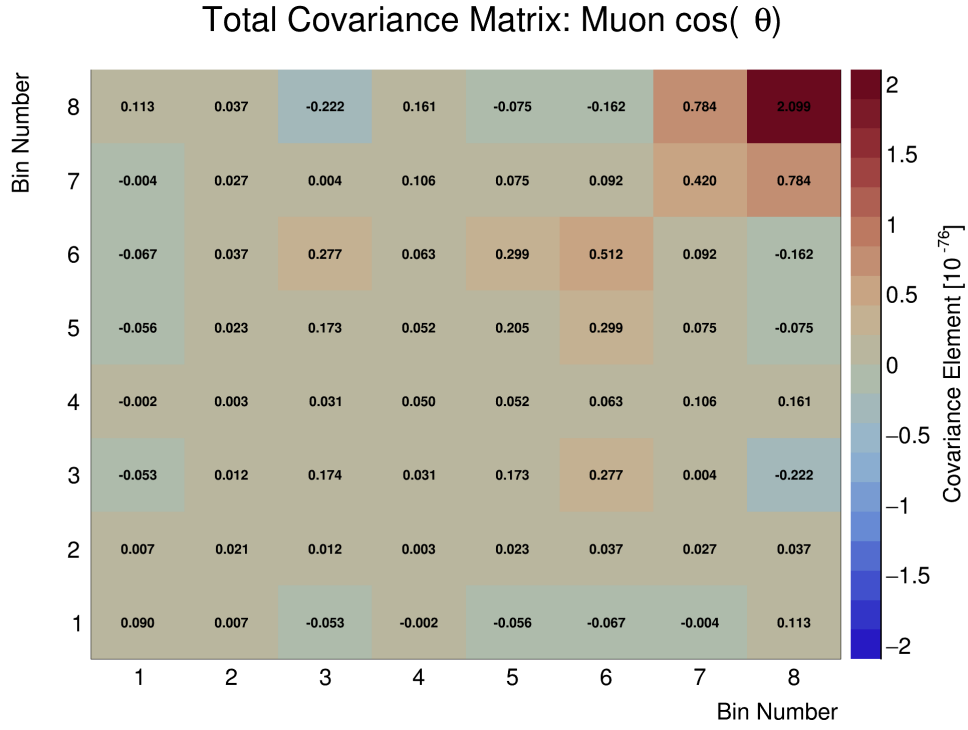

(b) Muon  $\cos(\theta_\mu)$

Figure 4: Covariance matrices for (a) the momentum of the muon and (b) the angle with respect to the beam,  $\cos(\theta)$ , of the muon.

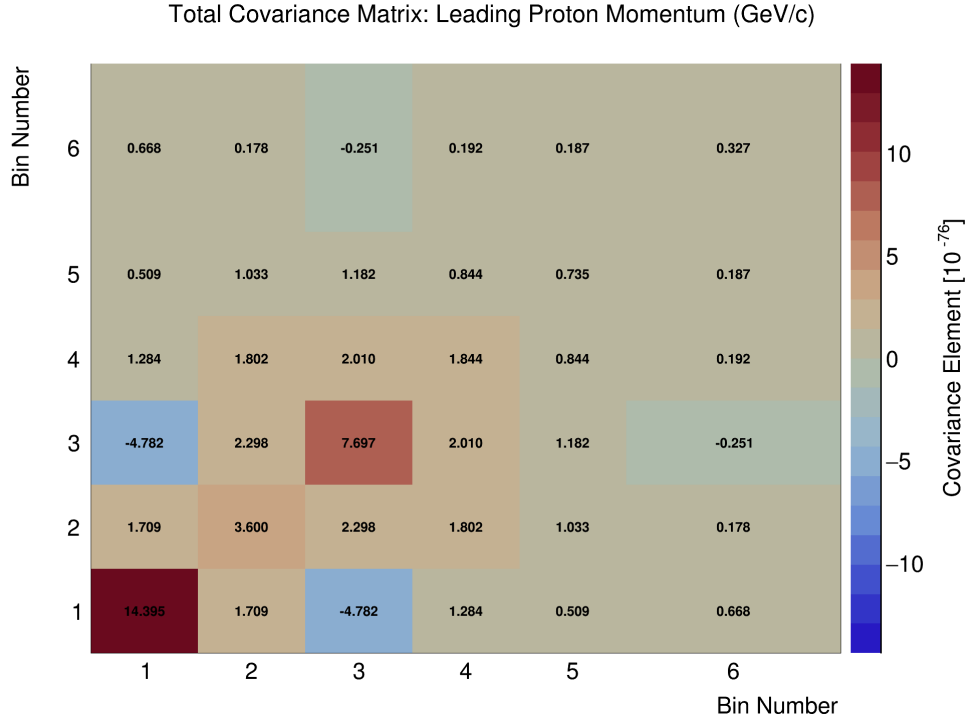

(a) Lead Proton Momentum,  $P_L$

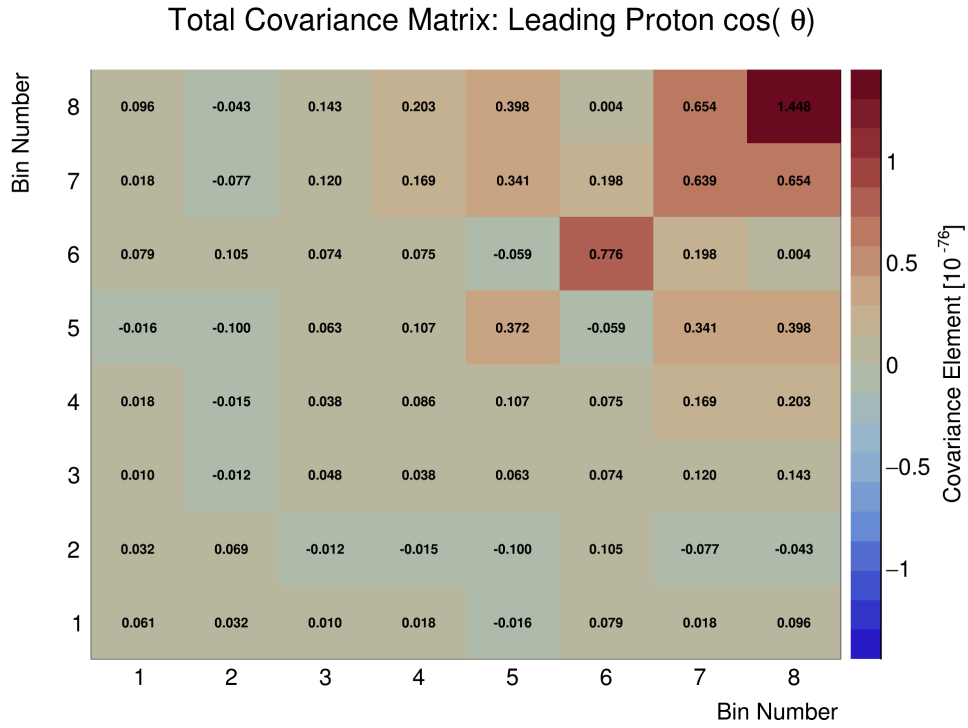

(b) Lead Proton  $\cos(\theta_L)$

Figure 5: Covariance matrices for (a) the momentum of the leading proton and (b) the angle with respect to the beam,  $\cos(\theta)$ , of the leading proton.

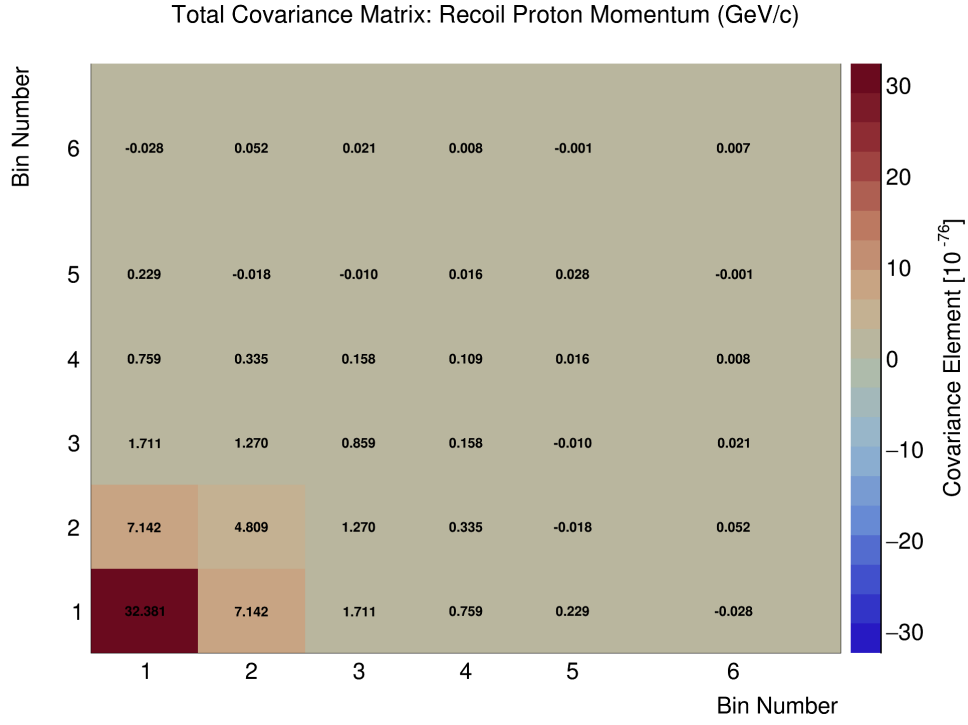

(a) Recoil Proton Momentum,  $P_R$

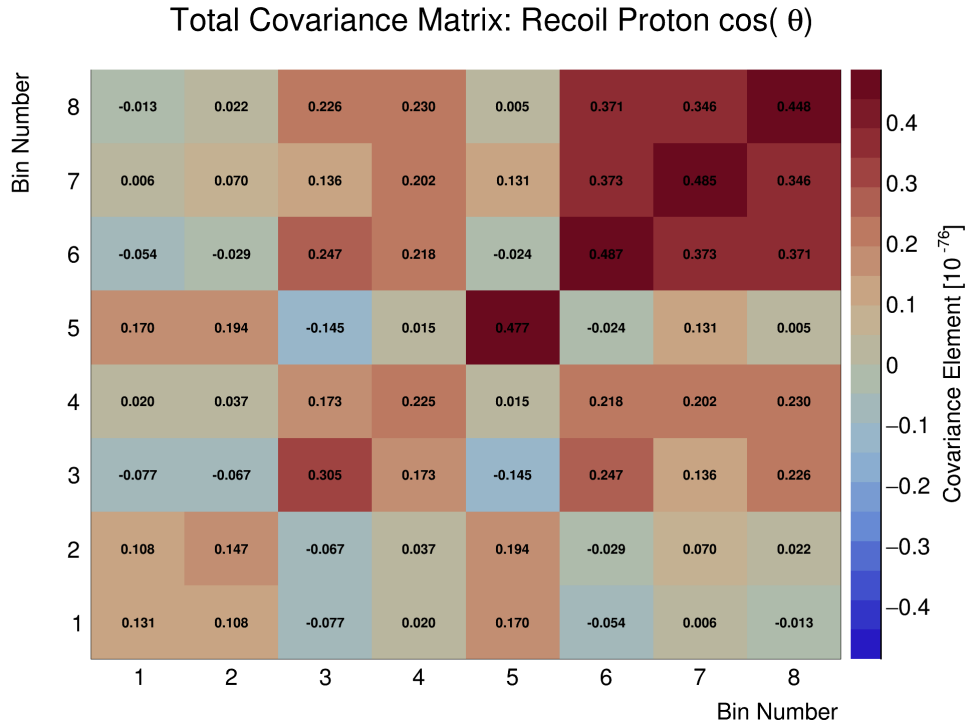

(b) Recoil Proton  $\cos(\theta_R)$

Figure 6: Covariance matrices for (a) the momentum of the recoil proton and (b) the angle with respect to the beam,  $\cos(\theta)$ , of the recoil proton.
